# Supplementary material for: Price of liquidity in the reinsurance of fund returns
Source: arXiv:2011.13268 source file (2020-11-26)
Supplement: Supplementary file 1 [file appendix.tex]

\section*{Appendix A: Baum-Welch \& HFRX Indices}
We use the well-known Baum-Welch algorithm to obtain plausible parameters for our Markov-switching simulation. As initial value for the Maximum likelihood estimation according to \textcite{baum1970maximization} we use the heuristic from \textcite{ernst2009portfolio} and compute the most likely sequence of states by means of Viterbi's algorithm from \textcite{viterbi1967error}. Figure \ref{HFRXEH} illustrates the resulting crisis periods for the HFRXEH index using the heuristic and the Baum-Welch algorithm created by the R-routine 'BaumWelch'. Table \ref{table HFRXEH} gives an overview on all analyzed HFRX indices and their respective parameters.

\begin{figure}[H]
\includegraphics[width = \textwidth]{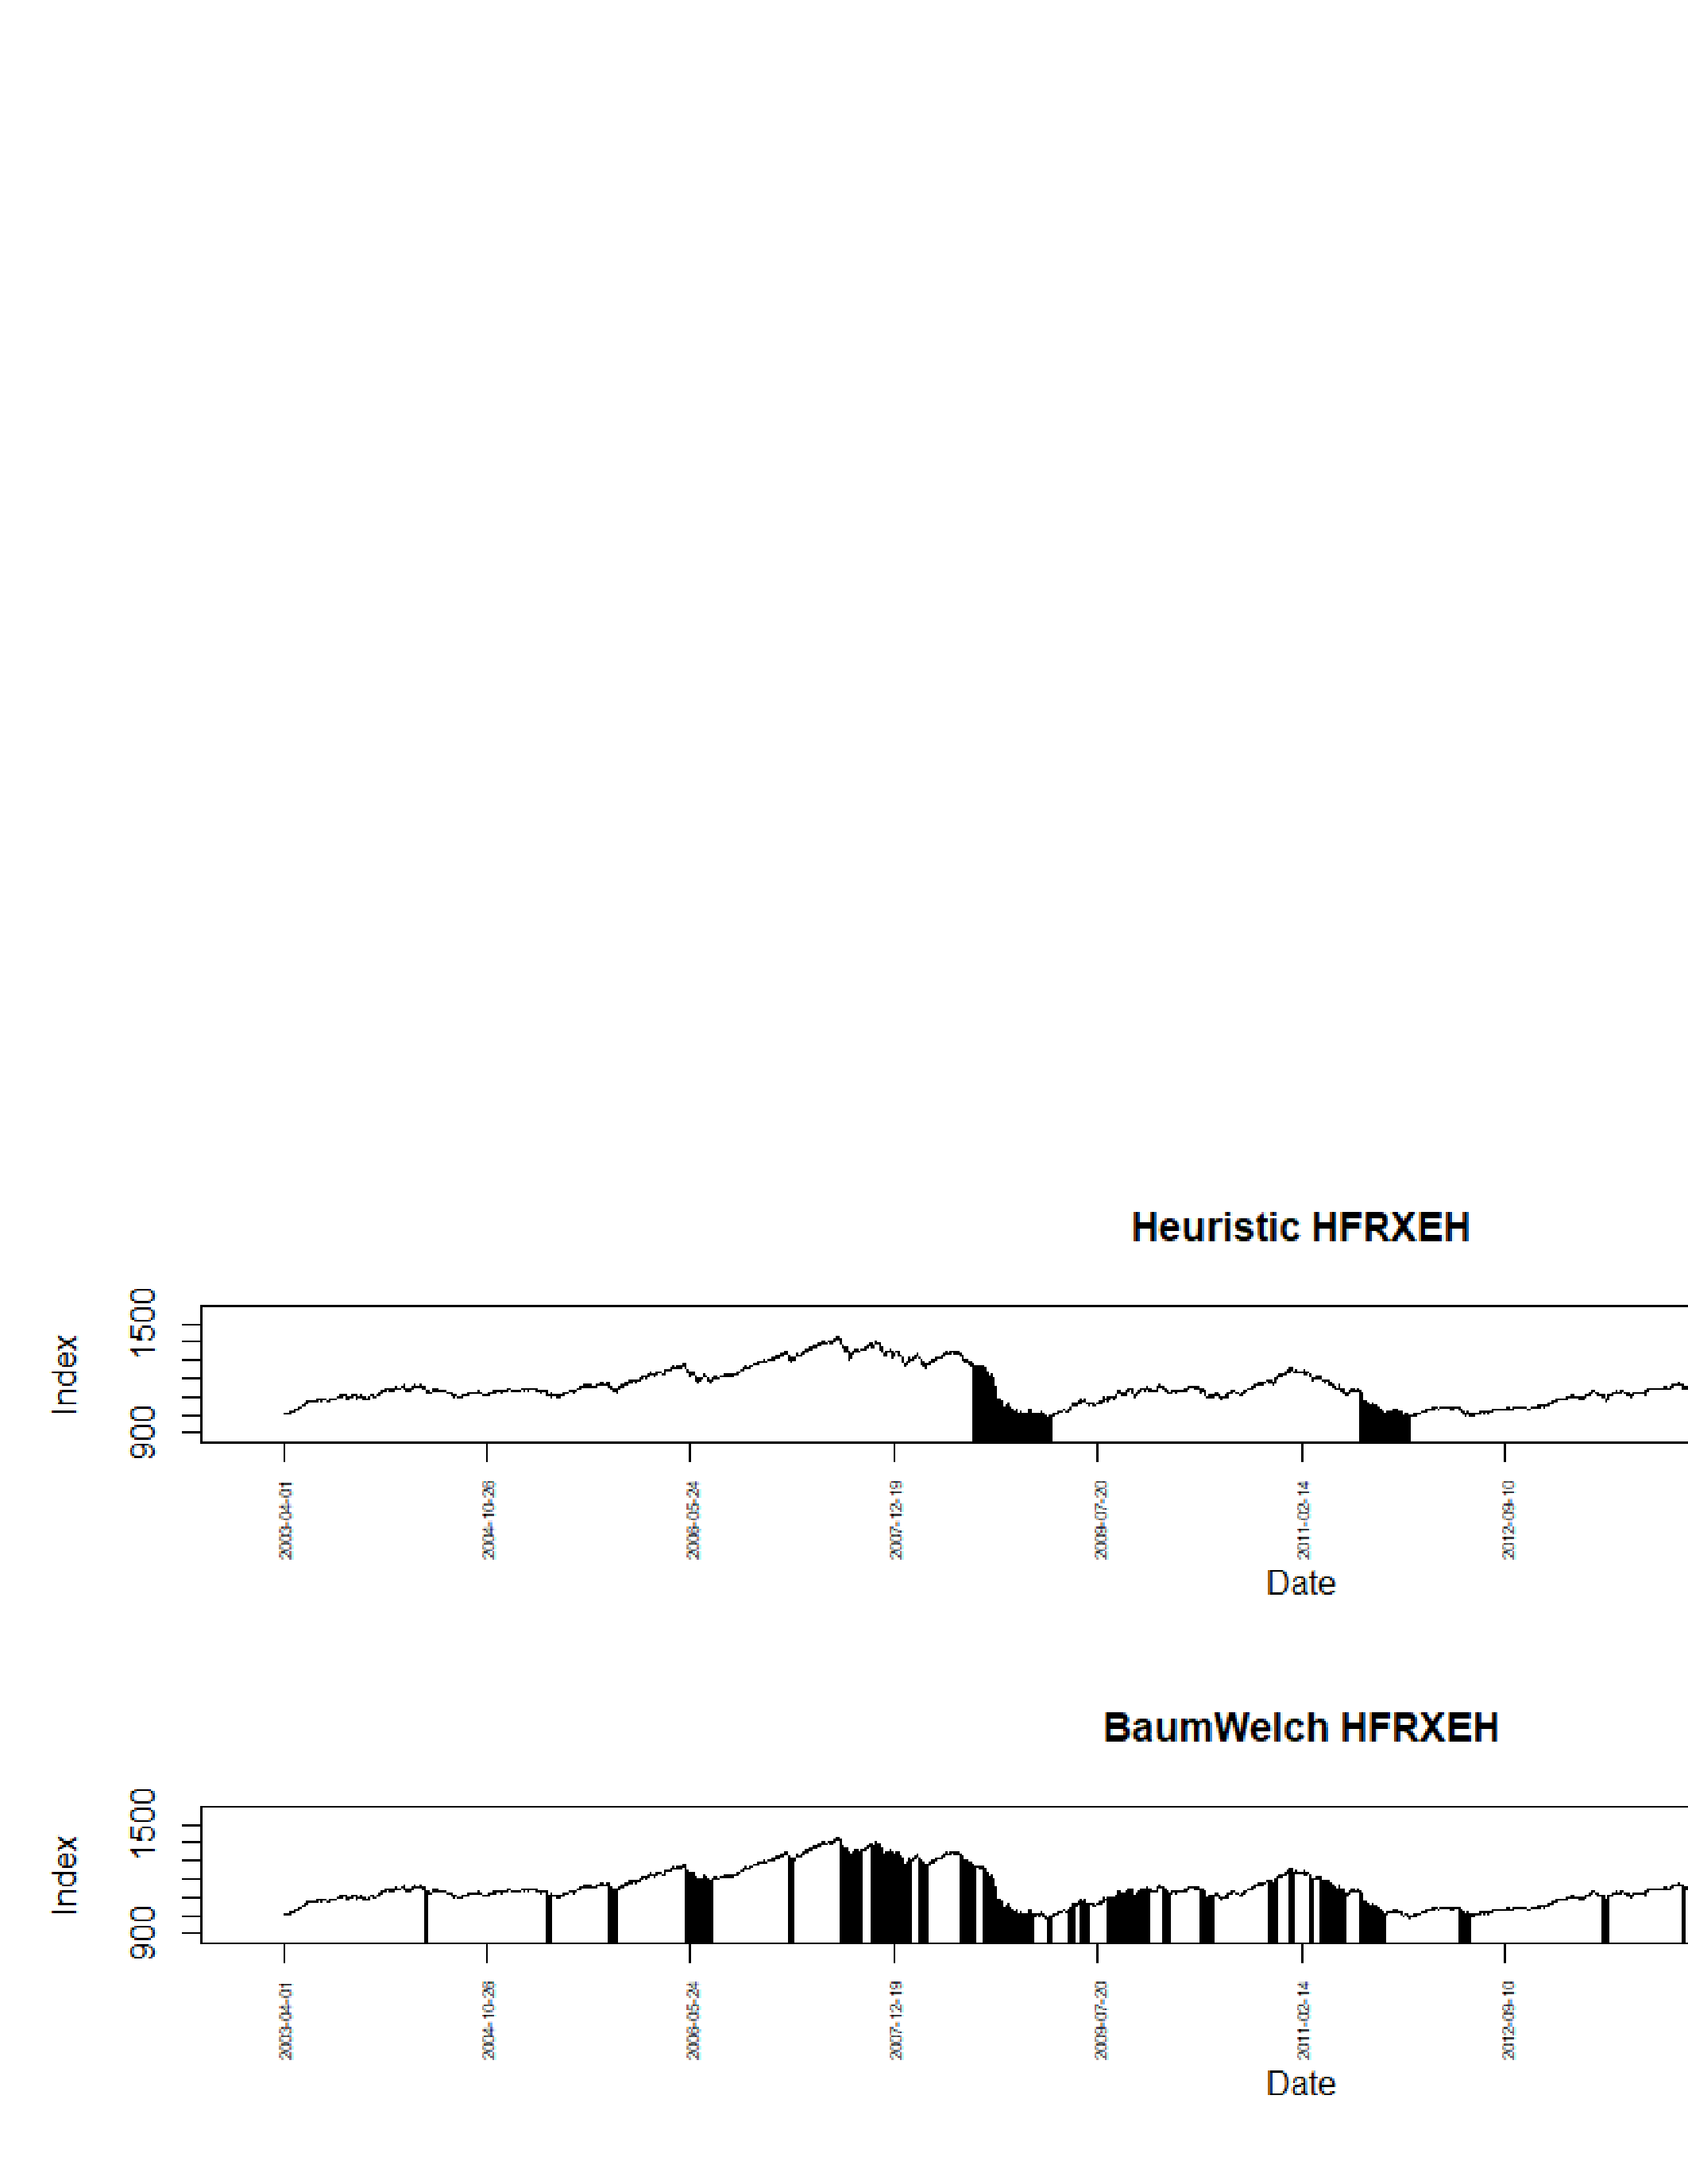}
\textit{This figure illustrates the HFRXEH Equity Hedge Index between April 1, 2003 and December 28, 2018. The top graph shows crisis periods in red using the crisis detection heuristic and the bottom graph shows crisis periods in blue using the Baum-Welch algorithm.}
\caption{HFRXEH}
\label{HFRXEH}
\end{figure}

\begin{table}[H]
\centering
\resizebox{\textwidth}{!}{\begin{tabular}{|lllcccccc|}
	\hline    
    Ticker & Index Name & Strategy & $p$ [in $\%$] & $q$ [in $\%$] & $\mu_1$ [in $\%$] & $\mu_2$ [in $\%$] & $\sigma_1$ [in $\%$] & $\sigma_2$ [in $\%$]\\
    \hline
    HFRXGL & HFRX Global Hedge Fund Index & Global & 1.67 & 7.49 & 8.54 & -32.40 & 2.57 & 6.44 \\
    HFRXM & HFRX Macro\textbackslash CTA Index & Macro & 1.87 & 7.79 & 4.84 & -15.36 & 4.55 & 10.93 \\
    HFRXEMN & HFRX EH: Equity Market Neutral Index & Neutral & 1.13 & 6.09 & 1.12 & -6.87 & 2.88 & 7.08 \\
    HFRXEH & HFRX Equity Hedge Index & Equity Hedge & 2.02 & 6.19 & 11.25 & -30.36 & 4.28 & 10.12 \\
    HFRXMA & HFRX ED: Merger Arbitrage Index & Merger Arbitrage & 2.07 & 15.70 & 5.46 & -8.27 & 2.16 & 10.17 \\
    \hline
    mean  &   &   & 1.75 & 8.65 & 6.24 & -18.65 & 3.29 & 8.95 \\
    max   &   &   & 2.07 & 15.70 & 11.25 & -6.87 & 4.55 & 10.93 \\
    min   &   &   & 1.13 & 6.09 & 1.12 & -32.40 & 2.16 & 6.44 \\
    \hline
    \end{tabular}}
 \textit{This table shows an overview on all HFRX indices and respective parameters obtained from the Baum-Welch algorithm.}
\caption{Overview HFRX}     
\label{table HFRXEH}

\end{table}
